# Supplementary material for: Analyzing ChatGPT's Aptitude in an Introductory Computer Engineering Course
Source: arXiv:2304.06122 source file (2023-04-14)
Supplement: Supplementary file 1 [file appendix.tex]

\appendices
\section{}
